# Supplementary material for: Linguistically-Informed Neural Architectures for Lexical, Syntactic and Semantic Tasks in Sanskrit
Source: arXiv:2308.08807 source file (2023-08-17)
Supplement: Supplementary file 1 [file AppendixTemplate.tex]

% Appendix Template

\chapter{Appendix Title Here} % Main appendix title

\label{AppendixX} % Change X to a consecutive letter; for referencing this appendix elsewhere, use \ref{AppendixX}

\lhead{Appendix X. \emph{Appendix Title Here}} % Change X to a consecutive letter; this is for the header on each page - perhaps a shortened title

Write your Appendix content here.
